# Supplementary material for: Learning Representations For Images With Hierarchical Labels
Source: arXiv:2004.00909 source file (2020-04-11)
Supplement: Supplementary file 1 [file appendix.tex]

\chapter{Appendix}
